# Supplementary material for: Less Is More: Tuning Configurable Systems with Imperfect Fidelity
Source: arXiv:2608.00759 source file (2026-08-01)
Supplement: Supplementary file 2 [file section_algorithm.tex]

% \tao{the flow is not very clear - I suggest to either start with a clear section to talk about GA/NSGA-II as it is, and then talk in our context how they are tailored (1. GA and NSGAII; GA and NSGAII in MFtune); or, we talk within our context directly (NSGAII in MFtune/GA in MFtune). The current structure is kind of too mix together. Could you give a overall section for this? e.g., detailed algorithm elaboration;, the 2nd part can be the current experiment.}

\section{Detailed Algorithm Elaboration}


\subsection{NSGA-II in \approach}

\subsubsection{Multi-objective Optimization}

A Multi-objective Optimization Problem (MOP) aims to optimize multiple conflicting objectives simultaneously.  
Formally, an MOP can be expressed as:
\begin{equation}
\begin{aligned}
    \arg \min \quad & \mathbf{F}(\boldsymbol{x}) = [f_1(\boldsymbol{x}),\, f_2(\boldsymbol{x}),\, \ldots,\, f_m(\boldsymbol{x})]^{T}, \\
    \text{s.t.} \quad & \boldsymbol{x} \in \Omega = \prod_{i=1}^{d} [L_i,\, U_i],
\end{aligned}
\label{eq:mop}
\end{equation}
where $\boldsymbol{x} = (x_1, \ldots, x_d)$ is a decision vector in the $d$-dimensional decision space $\Omega$, and  
$L_i$ and $U_i$ denote the lower and upper bounds of decision variable $x_i$, respectively.  
The vector $\mathbf{F}(\boldsymbol{x})$ contains $m$ objective functions, which are typically conflicting, making the problem inherently challenging.

\paragraph{Dominance and Non-dominance.}  
Given two solutions $\boldsymbol{x}_1$ and $\boldsymbol{x}_2$, $\boldsymbol{x}_1$ is said to \emph{dominate} $\boldsymbol{x}_2$ if: (1) it is no worse in all objectives, and (2) strictly better in at least one objective.  
If neither solution dominates the other, they are said to be \emph{non-dominated} with respect to each other.


\paragraph{Pareto Front.}  
All non-dominated solutions within a population form the \emph{Pareto front}.  
These solutions represent optimal trade-offs where improving one objective inevitably worsens at least one other.

\begin{figure}[h]
    \centering
    \includegraphics[width=0.5\linewidth]{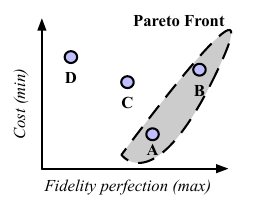}
    \caption{Illustration of dominance relationships.}
    \label{fig:nondominance}
\end{figure}

In this work, \approach~formulated the imperfect-fidelity discovering as a multi-objective optimization problem that maximizes fidelity perfection while minimizing measurement cost. As an example, illustrated in Figure~\ref{fig:nondominance}, where each point represents a fidelity setting, with cost plotted on the vertical axis and fidelity perfection on the horizontal axis. Under these two objectives, the fidelity setting ``D'' is dominated by ``A'', ``B'', and ``C'' because it is worse in both objectives. Fidelity setting ``C'' is dominated by ``A'', since ``A'' achieves both lower cost and higher fidelity perfection. In contrast, ``A'' and ``B'' do not dominate each other---``A'' achieves lower cost while ``B'' achieves higher perfection---so both appear on the Pareto front as mutually non-dominated trade-offs.



\subsubsection{NSGA-II}
To address the above multi-objective optimization problem and effectively balance the trade-off between fidelity perfection and cost, \approach~adopts the well-established NSGA-II, which is a widely used multi-objective genetic algorithm that combines Pareto-based ranking with a diversity-preserving selection. Its environmental selection is driven by two key ideas: fast non-dominated sorting and crowding distance~\cite{deb2002fast}.

\paragraph{Fast Non-dominated Sorting.}
The combined population of parent and offspring is partitioned into a sequence of Pareto fronts based on dominance. The first front contains all
solutions that are not dominated by any other solution in the
population (the current Pareto front). The second front contains all
solutions that are only dominated by members of the first front, the
third front contains solutions dominated only by members of the first
two fronts, and so on. This yields an ordered hierarchy of fronts with
increasing dominance level. Figure~\ref{fig:fast} illustrates this idea.

\begin{figure}[h]
    \centering
    \includegraphics[width=0.5\linewidth]{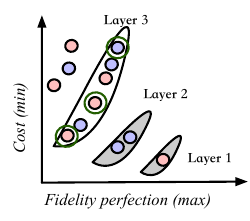}
    \caption{Illustration of fast non-dominated sorting in the objective space.}
    \label{fig:fast}
\end{figure}

\paragraph{Crowding distance.}
To maintain diversity within each Pareto front, NSGA-II assigns every
solution a crowding distance that estimates how isolated it is from its
neighbors in objective space. For each front, solutions are sorted
along each objective, boundary points are given an infinite distance,
and interior points receive the (normalized) distance to their nearest
neighbors. 

% \textbf{Illustration in this work.}

\paragraph{Imperfect-Fidelity Discovering.} In this study, we formulate imperfect-fidelity discovering as a multi-objective problem (maximizing fidelity perfection and minimizing cost), which is optimized using NSGA-II. Specifically, it explores the fidelity space by evolving candidate fidelity settings via selection, crossover, and mutation operators (details in \S\ref{subsection:ga_mftune}). To handle the trade-off between cost and fidelity perfection, fast non-dominated sorting and crowding distance are employed to select the population for the next generation. As illustrated in Figure~\ref{fig:fast}, parent (blue) and offspring (red) solutions (i.e., fidelity settings) are first merged and sorted into Pareto fronts. Then, the population of the next generation is filled by taking whole fronts in order of rank until adding the next front would exceed the population size. If the last admissible front does not fit entirely, solutions in that front are sorted by crowding distance and the most isolated ones are selected (e.g., the green-circled points in Figure~\ref{fig:fast}).

 % \item \textbf{Imperfect-Fidelity Discovering:} GA explores the fidelity space by evolving candidate fidelity settings via selection, crossover, and mutation. To handle the trade-off between cost and fidelity perfection, NSGA-II is employed as the environmental selection mechanism, allowing GA to identify a fair fidelity setting that offers a high level of fidelity perfection at low cost.

\subsection{GA in \approach}
\label{subsection:ga_mftune}
Genetic Algorithm (GA)~\cite{back1993overview} is a population-based metaheuristic inspired by natural evolution. Starting from an initial population of candidate solutions, GA repeatedly applies genetic operators( i.e., selection, crossover, and mutation) to evolve the population toward higher quality solutions. In each iteration (generation), parent solutions are selected based on a selection operator and recombined through crossover, followed by mutation, to produce a set of offspring. The offspring are then merged with the current population, and an environmental selection is applied to choose the next population, often favoring fitter and more diverse individuals. This iterative process continues until a termination criterion is met, such as reaching a fixed number of generations or convergence of the population. Figure~\ref{fig:ga} illustrates the conventional GA workflow.

In \approach, GA is employed in two components, i.e., finding seeds under imperfect-fidelity and assuring under perfect-fidelity with seeds:

\begin{itemize}
    \item \textbf{Imperfect-fidelity Seeding:} Once the fair imperfect-fidelity setting is chosen, GA evolves candidate configurations under this inexpensive fidelity setting, achieving wide exploration. Environmental selection is now based solely on configuration performance, iteratively recombining and mutating configurations to obtain strong configuration seeds for the subsequent stage.
    \item \textbf{Perfect-fidelity Assuring:} GA then evaluates and refines the seeded configuration under the perfect-fidelity setting, performing depth tuning.
\end{itemize}


% \begin{itemize}
%     \item \textbf{Imperfect-Fidelity Discovering:} GA evolves candidate fidelity settings via crossover and mutation to search for a fidelity setting that achieves a high level of fidelity perfection at low cost---a ``fair'' imperfect-fidelity setting that serves as an efficient proxy for perfect-fidelity.
%     \item \textbf{Imperfect-fidelity Seeding:} GA evolves candidate configurations under the chosen fidelity setting (imperfect- or perfect-fidelity setting), iteratively recombining and mutating configurations to identify those that yield the best performance (e.g., throughput and runtime).
%     \item \textbf{Perfect-fidelity Assuring:}
% \end{itemize}

These two uses of GA allow \approach~to efficiently explore the configuration space.

\begin{figure}[t]
    \centering
    \includegraphics[width=0.75\linewidth]{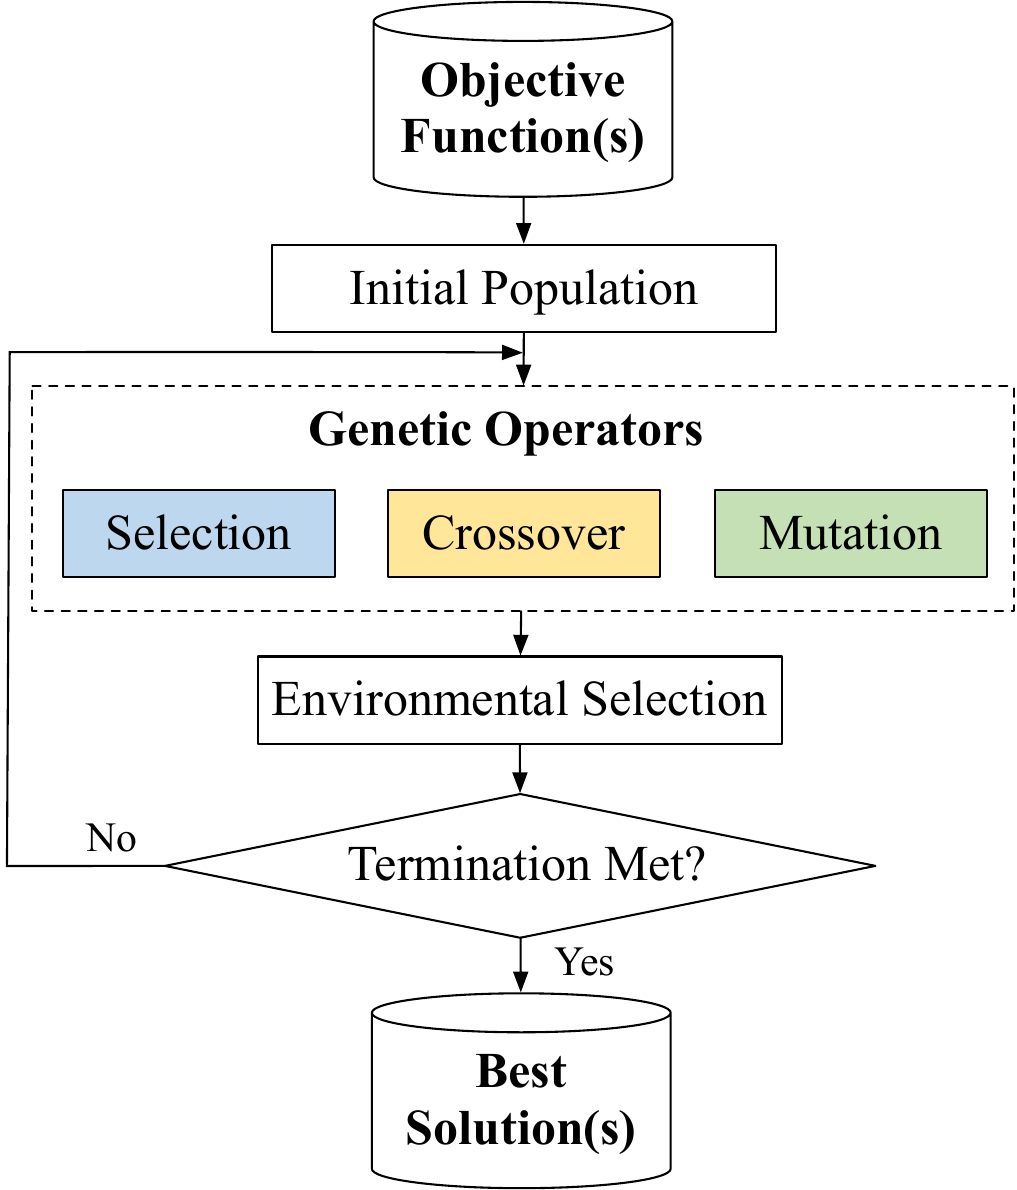}
    \caption{The workflow of genetic algorithm.}
    \label{fig:ga}
\end{figure}

% \subsection{Uniform Crossover Operator}
\paragraph{Uniform Crossover Operator}

% Uniform crossover recombines two parent solutions by independently deciding, for each decision variable, which parent contributes the value, i.e., flipping a fair coin (with probability 0.5) for each dimension $i$. For example, given two parents $\boldsymbol{x}^1$ = \{$x^{1}_{1}, x^{1}_{2}, \dots, x^{1}_{d}$\} and $\boldsymbol{x}^2$ = \{$x^{2}_{1}, x^{2}_{2}, \dots, x^{2}_{d}$\}, the operator generates offspring $\boldsymbol{o}^1$ = \{$o^{1}_{1}, o^{1}_{2}, \dots, o^{1}_{d}$\} and $\boldsymbol{o}^2$ = \{$o^{2}_{1}, o^{2}_{2}, \dots, o^{2}_{d}$\} where: 

% \begin{equation}
% o^{1}_{i} =
% \begin{cases}
% x^{1}_i, & \text{if } u_i \textless 0.5,\\[4pt]
% x^{2}_i, & \text{if } u_i \ge 0.5.
% \end{cases}
% \end{equation}

% \begin{equation}
% o^{2}_{i} =
% \begin{cases}
% x^{2}_i, & \text{if } u_i \textless 0.5,\\[4pt]
% x^{1}_i, & \text{if } u_i \ge 0.5.
% \end{cases}
% \end{equation}


Uniform crossover recombines two parent solutions by independently deciding, for each decision variable, whether the values of the two parents should be exchanged.
Given two parents $\boldsymbol{x}^{1}=\{x^{1}_1,\ldots,x^{1}_d\}$ and $ \boldsymbol{x}^{2}=\{x^{2}_1,\ldots,x^{2}_d\}$, the operator produces two offspring
$\boldsymbol{o}^{1}=\{o^{1}_1,\ldots,o^{1}_d\}$ and
$\boldsymbol{o}^{2}=\{o^{2}_1,\ldots,o^{2}_d\}.$ For each dimension $i$, a random number $u_i\sim \mathbfcal{U}(0,1)$ is sampled. 
With a probability of $0.5$, the values from the two parents are kept in the same order; otherwise, they are swapped:
\begin{equation}
\big(o^{1}_i,\, o^{2}_i\big)=
\begin{cases}
\big(x^{1}_i,\, x^{2}_i\big), & \text{if } u_i < 0.5,\\[6pt]
\big(x^{2}_i,\, x^{1}_i\big), & \text{if } u_i \ge 0.5.
\end{cases}
\label{eq:uniform-crossover}
\end{equation}

This dimension-wise decision ensures that each variable of the offspring 
is independently inherited from either parent with equal probability. 
Figure~\ref{fig:crossover} illustrates this process.



\begin{figure}[h]
    \centering
    \includegraphics[width=0.5\linewidth]{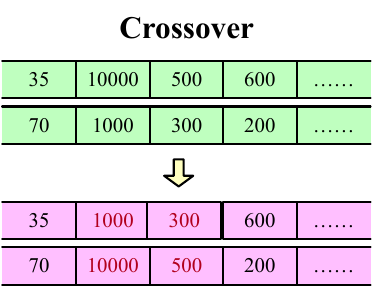}
    \caption{Illustration of the uniform crossover operator, where each variable is independently inherited from either parent with equal probability.}
    \label{fig:crossover}
\end{figure}

% \subsection{Boundary Mutation Operator}
\paragraph{Boundary Mutation Operator}

Boundary mutation perturbs a decision variable by randomly resampling its value within the feasible range. Given a solution $\boldsymbol{x}$ = $\{x_1,\ldots,x_d\}$,
each decision variable $x_i$ is associated with a lower bound $L_i$ and an upper bound $U_i$. During mutation, a variable is modified with a mutation probability, denoted as $\beta$.
Specifically, for each dimension $i$, a random number $u_i \sim \mathbfcal{U}(0,1)$
is drawn, and the mutated variable $x_i'$ is given by:

\begin{equation}
    x_i' = 
\begin{cases}
\text{Uniform}(L_i, U_i), & \text{if } u_i < \beta,\\[6pt]
x_i, & \text{otherwise}.
\end{cases}
\end{equation}

This resampling-based mutation ensures that any mutated value remains feasible
while enabling exploration across the entire valid range of the 
space. Figure~\ref{fig:mutation} illustrates this process, where a selected
variable is replaced by a new value sampled within its allowable range.

\begin{figure}[h]
    \centering
    \includegraphics[width=0.5\linewidth]{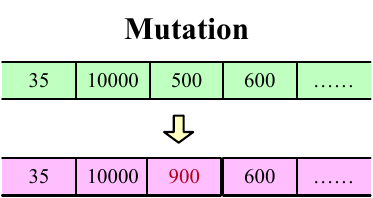}
    \caption{Illustration of the boundary mutation operator, where a selected variable is replaced by a randomly sampled feasible value.}
    \label{fig:mutation}
\end{figure}
