# Supplementary material for: Less Is More: Tuning Configurable Systems with Imperfect Fidelity
Source: arXiv:2608.00759 source file (2026-08-01)
Supplement: Supplementary file 3 [file section_ga.tex]

\tao{the flow is not very clear - I suggest to either start with a clear section to talk about GA/NSGA-II as it is, and then talk in our context how they are tailored (1. GA and NSGAII; GA and NSGAII in MFtune); or, we talk within our context directly (NSGAII in MFtune/GA in MFtune). The current structure is kind of too mix together. Could you give a overall section for this? e.g., detailed algorithm elaboration;, the 2nd part can be the current experiment.}


\subsection{GA in \approach}










% \subsection{Overview}
Genetic Algorithm (GA)~\cite{back1993overview} is a population-based metaheuristic inspired by natural evolution. Starting from an initial population of candidate solutions, GA repeatedly applies genetic operators( i.e., selection, crossover, and mutation) to evolve the population toward higher quality solutions. In each iteration (generation), parent solutions are selected based on a selection operator and recombined through crossover, followed by mutation, to produce a set of offspring. The offspring are then merged with the current population, and an environmental selection is applied to choose the next population, often favoring fitter and more diverse individuals. This iterative process continues until a termination criterion is met, such as reaching a fixed number of generations or convergence of the population. Figure~\ref{fig:ga} illustrates the conventional GA workflow.

\begin{figure}[h]
    \centering
    \includegraphics[width=0.75\linewidth]{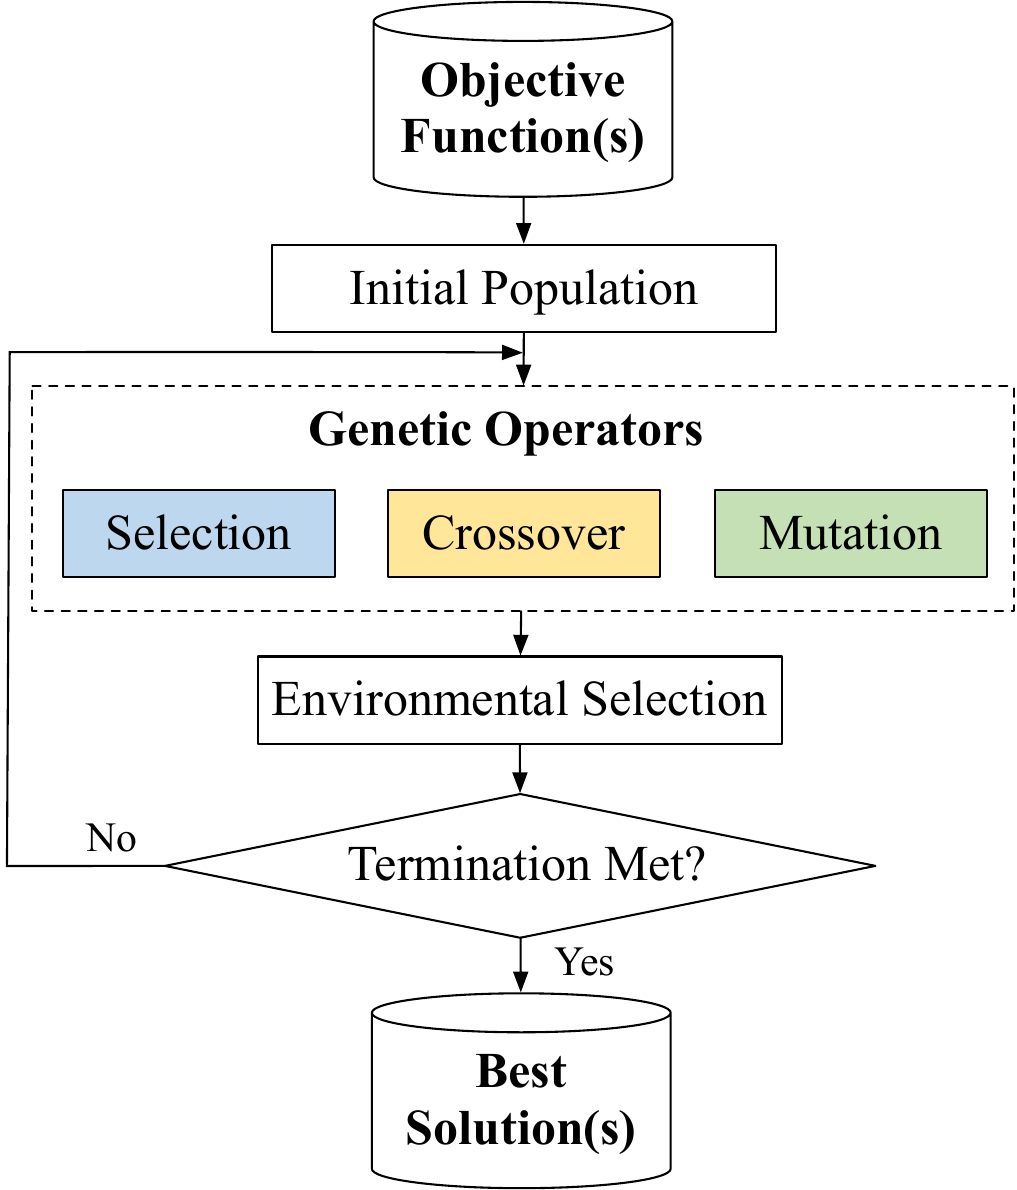}
    \caption{The workflow of genetic algorithm.}
    \label{fig:ga}
\end{figure}

% \subsection{Uniform Crossover Operator}
\paragraph{Uniform Crossover Operator}

% Uniform crossover recombines two parent solutions by independently deciding, for each decision variable, which parent contributes the value, i.e., flipping a fair coin (with probability 0.5) for each dimension $i$. For example, given two parents $\boldsymbol{x}^1$ = \{$x^{1}_{1}, x^{1}_{2}, \dots, x^{1}_{d}$\} and $\boldsymbol{x}^2$ = \{$x^{2}_{1}, x^{2}_{2}, \dots, x^{2}_{d}$\}, the operator generates offspring $\boldsymbol{o}^1$ = \{$o^{1}_{1}, o^{1}_{2}, \dots, o^{1}_{d}$\} and $\boldsymbol{o}^2$ = \{$o^{2}_{1}, o^{2}_{2}, \dots, o^{2}_{d}$\} where: 

% \begin{equation}
% o^{1}_{i} =
% \begin{cases}
% x^{1}_i, & \text{if } u_i \textless 0.5,\\[4pt]
% x^{2}_i, & \text{if } u_i \ge 0.5.
% \end{cases}
% \end{equation}

% \begin{equation}
% o^{2}_{i} =
% \begin{cases}
% x^{2}_i, & \text{if } u_i \textless 0.5,\\[4pt]
% x^{1}_i, & \text{if } u_i \ge 0.5.
% \end{cases}
% \end{equation}


Uniform crossover recombines two parent solutions by independently deciding, for each decision variable, whether the values of the two parents should be exchanged.
Given two parents $\boldsymbol{x}^{1}=\{x^{1}_1,\ldots,x^{1}_d\}$ and $ \boldsymbol{x}^{2}=\{x^{2}_1,\ldots,x^{2}_d\}$, the operator produces two offspring
$\boldsymbol{o}^{1}=\{o^{1}_1,\ldots,o^{1}_d\}$ and
$\boldsymbol{o}^{2}=\{o^{2}_1,\ldots,o^{2}_d\}.$ For each dimension $i$, a random number $u_i\sim \mathbfcal{U}(0,1)$ is sampled. 
With a probability of $0.5$, the values from the two parents are kept in the same order; otherwise, they are swapped:
\begin{equation}
\big(o^{1}_i,\, o^{2}_i\big)=
\begin{cases}
\big(x^{1}_i,\, x^{2}_i\big), & \text{if } u_i < 0.5,\\[6pt]
\big(x^{2}_i,\, x^{1}_i\big), & \text{if } u_i \ge 0.5.
\end{cases}
\label{eq:uniform-crossover}
\end{equation}

This dimension-wise decision ensures that each variable of the offspring 
is independently inherited from either parent with equal probability. 
Figure~\ref{fig:crossover} illustrates this process.



\begin{figure}[h]
    \centering
    \includegraphics[width=0.5\linewidth]{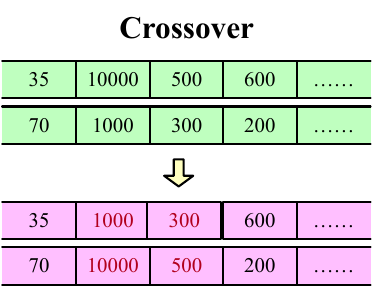}
    \caption{Illustration of the uniform crossover operator, where each variable is independently inherited from either parent with equal probability.}
    \label{fig:crossover}
\end{figure}

% \subsection{Boundary Mutation Operator}
\paragraph{Boundary Mutation Operator}

Boundary mutation perturbs a decision variable by randomly resampling its value within the feasible range. Given a solution $\boldsymbol{x}$ = $\{x_1,\ldots,x_d\}$,
each decision variable $x_i$ is associated with a lower bound $L_i$ and an upper bound $U_i$. During mutation, a variable is modified with a mutation probability, denoted as $\beta$.
Specifically, for each dimension $i$, a random number $u_i \sim \mathbfcal{U}(0,1)$
is drawn, and the mutated variable $x_i'$ is given by:

\begin{equation}
    x_i' = 
\begin{cases}
\text{Uniform}(L_i, U_i), & \text{if } u_i < \beta,\\[6pt]
x_i, & \text{otherwise}.
\end{cases}
\end{equation}

This resampling-based mutation ensures that any mutated value remains feasible
while enabling exploration across the entire valid range of the 
space. Figure~\ref{fig:mutation} illustrates this process, where a selected
variable is replaced by a new value sampled within its allowable range.

\begin{figure}[h]
    \centering
    \includegraphics[width=0.5\linewidth]{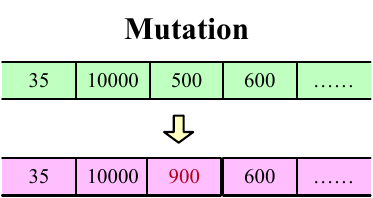}
    \caption{Illustration of the boundary mutation operator, where a selected variable is replaced by a randomly sampled feasible value.}
    \label{fig:mutation}
\end{figure}
