# Supplementary material for: Less Is More: Tuning Configurable Systems with Imperfect Fidelity
Source: arXiv:2608.00759 source file (2026-08-01)
Supplement: Supplementary file 4 [file section_guideline.tex]

\section{How to Use \approach~on a New System?}
\approach~is designed to support a wide range of configurable systems with minimal system-specific effort. Integrating a new system requires only lightweight modifications to a few system-facing interfaces, after which \approach~can directly orchestrate the tuning process. In the remainder of this section, we describe step by step how a new system can be incorporated into \approach, from specifying the system interface to defining configuration options, fidelity settings, and the necessary controller.

\subsection{Step 1: Specify the Target System}
To integrate a new system into \approach, the practitioner should first specify the basic system information and how \approach~will interact with it.

This step typically involves the following aspects:

\begin{itemize}
    \item \textbf{System name and version:} Specify the exact software name and version to be tuned.
    \item \textbf{Deployment mode:} \approach~supports various deployment modes (local execution, remote services, or Docker containers); we strongly recommend using Docker for consistency and isolation.
    \item \textbf{System interfaces:} A custom \texttt{System} class defines how \approach~applies and retrieves configuration options, and how the system is started, stopped, or reset. \approach’s modular design allows developers to implement them with minimal effort.
\end{itemize}

\subsection{Step 2: Define Configuration Options}
Next, the practitioner should define a set of tunable configuration options that may influence the system's performance. These options can be obtained from system manual, tuning guides, or prior work on configuration tuning. Each option is then described by its \texttt{name}, \texttt{type}, and \texttt{domain}, and encoded in a small configuration specification that \approach~can process uniformly.

For example, the following illustrates how \textsc{Httpd}'s configuration options can be defined in \texttt{JSON}:

\begin{minipage}{\linewidth}
\begin{minted}[fontsize=\small,breaklines,frame=single]{json}
{   "TimeOut": {
    "default": 60,
    "min": 1,
    "max": 600,
    "type": "integer"
  },
  "KeepAlive": {
    "default": "On",
    "enum_values": ["Off", "On"],
    "type": "enum"
  },
  ...
}
\end{minted}
\end{minipage}

\subsection{Identify Fidelity Generators/Factors}
To conveniently control the fidelity setting (measurement environment), \approach\ relies on fidelity generators such as benchmark tools. A fidelity generator (e.g., \textsc{Sysbench} for database) exercises the target system under a configurable environment, while a set of fidelity factors exposes how this environment can be varied (e.g., workload intensity, duration, or concurrency). These factors allow practitioners to construct multiple fidelity settings---either by using existing benchmark parameters or by manually designing a family of environments---without changing the core tuning logic.

For each fidelity factor, we specify its \texttt{name}, \texttt{type}, and \texttt{domain}. In addition, we designate a target perfect-fidelity setting, which represents the environment under which the system should be tuned. 

The following example shows how \textsc{Wrk}'s fidelity factors can be defined in \texttt{JSON} for web servers:


\begin{minipage}{\linewidth}
\vspace{4pt}
\begin{minted}[fontsize=\small,breaklines,frame=single]{json}
{   "connections": {
    "default": 50,
    "type": "enum",
    "enum_values": [10, 15, 20, 25, 30, 35, 40, 45, 50]
  },
  "duration": {
    "default": 180,
    "type": "enum",
    "enum_values": [10, 15, 20, 25, 30, 35, 40, 45, 50, 55, 60]
  },
  ...
}
\end{minted}
\vspace{2pt}
\end{minipage}

Here, the \texttt{default} values jointly define the target perfect-fidelity setting.

\subsection{Realize the Environment Controller}
The fourth step is to implement an environment controller that defines how the system is executed and evaluated under a given fidelity setting. This controller prepares a clean evaluation environment, applies the desired fidelity factors, invokes the corresponding workload, and captures the resulting performance measurements. Depending on the system, this may involve resetting the service, cleaning residual state, or re-initializing data before each run. Our modular design keeps this component lightweight: developers only need to implement a small interface that, given a fidelity specification, executes the system and returns the performance metric to be optimized.

By completing the steps above and implementing the required lightweight interfaces, a new system can be seamlessly integrated into \approach. More implementation/deployment details can be found in our repository: \textcolor{blue}{\texttt{\url{https://github.com/ideas-labo/mftune}}}. 



























\begin{table*}[htbp]
    \centering
    \small
    \setlength{\tabcolsep}{18pt}
    \caption{Details of configuration options of \textsc{MySQL}.}
 %    \begin{adjustbox}{width=\linewidth,center}
	% \begin{threeparttable}
		\input{supplementary/sup_figures/mysql_knobs_table}
	% \end{threeparttable}
 %    \end{adjustbox}
    \label{tab:mysql}
\end{table*}


\begin{table*}[htbp]
    \centering
    \small
        \setlength{\tabcolsep}{18pt}
    \caption{Details of configuration options of \textsc{Httpd}.}
 %    \begin{adjustbox}{width=\linewidth,center}
	% \begin{threeparttable}
		\input{supplementary/sup_figures/httpd_knobs_table}
	% \end{threeparttable}
 %    \end{adjustbox}

    \label{tab:httpd}
\end{table*}

\clearpage

\begin{table}[htbp]
    \centering
        \small
    \caption{Details of configuration options of \textsc{PostgreSQL}.}
    \begin{adjustbox}{width=\linewidth,center}
	\begin{threeparttable}
\input{supplementary/sup_figures/postgresql_knobs_table}
	\end{threeparttable}
    \end{adjustbox}
    \label{tab:postgresql}
\end{table}

\begin{table}[htbp]
    \centering
        \small
    \caption{Details of configuration options of \textsc{Tomcat}.}
    \begin{adjustbox}{width=\linewidth,center}
	\begin{threeparttable}
\input{supplementary/sup_figures/tomcat_knobs_table}
	\end{threeparttable}
    \end{adjustbox}
    \label{tab:tomcat}
\end{table}


\begin{table}[htbp]
    \centering
        \small
    \caption{Details of configuration options of \textsc{Gcc}.}
    \begin{adjustbox}{width=\linewidth,center}
	\begin{threeparttable}
		\input{supplementary/sup_figures/gcc_knobs_table}
	\end{threeparttable}
    \end{adjustbox}

    \label{tab:gcc}
\end{table}

\begin{table}[htbp]
    \centering
        \small
    \caption{Details of configuration options of \textsc{Clang}.}
    \begin{adjustbox}{width=\linewidth,center}
	\begin{threeparttable}
		\input{supplementary/sup_figures/clang_knobs_table}
	\end{threeparttable}
    \end{adjustbox}

    \label{tab:clang}
\end{table}
