# Supplementary material for: Less Is More: Tuning Configurable Systems with Imperfect Fidelity
Source: arXiv:2608.00759 source file (2026-08-01)
Supplement: Supplementary file 5 [file section_mop.tex]

\subsection{Multi-objective Optimization in \approach}

A Multi-objective Optimization Problem (MOP) aims to optimize multiple conflicting objectives simultaneously.  
Formally, an MOP can be expressed as:
\begin{equation}
\begin{aligned}
    \arg \min \quad & \mathbf{F}(\boldsymbol{x}) = [f_1(\boldsymbol{x}),\, f_2(\boldsymbol{x}),\, \ldots,\, f_m(\boldsymbol{x})]^{T}, \\
    \text{s.t.} \quad & \boldsymbol{x} \in \Omega = \prod_{i=1}^{d} [L_i,\, U_i],
\end{aligned}
\label{eq:mop}
\end{equation}
where $\boldsymbol{x} = (x_1, \ldots, x_d)$ is a decision vector in the $d$-dimensional decision space $\Omega$, and  
$L_i$ and $U_i$ denote the lower and upper bounds of decision variable $x_i$, respectively.  
The vector $\mathbf{F}(\boldsymbol{x})$ contains $m$ objective functions, which are typically conflicting, making the problem inherently challenging.

\paragraph{Dominance and Non-dominance.}  
Given two solutions $\boldsymbol{x}_1$ and $\boldsymbol{x}_2$, $\boldsymbol{x}_1$ is said to \emph{dominate} $\boldsymbol{x}_2$ if: (1) it is no worse in all objectives, and (2) strictly better in at least one objective.  
If neither solution dominates the other, they are said to be \emph{non-dominated} with respect to each other.


\paragraph{Pareto Front.}  
All non-dominated solutions within a population form the \emph{Pareto front}.  
These solutions represent optimal trade-offs where improving one objective inevitably worsens at least one other.

\begin{figure}[h]
    \centering
    \includegraphics[width=0.5\linewidth]{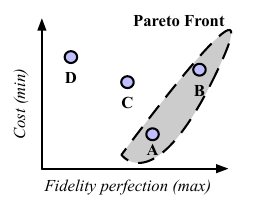}
    \caption{Illustration of dominance relationships.}
    \label{fig:nondominance}
\end{figure}

In this work, \approach~formulated the imperfect-fidelity discovering as a multi-objective optimization problem that maximizes fidelity perfection while minimizing measurement cost. As shown in Figure~\ref{fig:nondominance}, each point represents a fidelity setting, with cost plotted on the vertical axis and fidelity perfection on the horizontal axis.
Under these two objectives, the fidelity setting ``D'' is dominated by ``A'', ``B'', and ``C'' because it is worse in both objectives.
Fidelity setting C is dominated by ``A'' since ``A'' achieves both lower cost and higher fidelity perfection. In contrast, ``A'' and B do not dominate each other---``A'' achieves lower cost while ``B'' achieves higher perfection---so both appear on the Pareto front as mutually non-dominated trade-offs.
