# Supplementary material for: Less Is More: Tuning Configurable Systems with Imperfect Fidelity
Source: arXiv:2608.00759 source file (2026-08-01)
Supplement: Supplementary file 6 [file section_nsga-ii.tex]

\subsection{NSGA-II in \approach}

NSGA-II is a widely used multi-objective genetic algorithm that combines
Pareto-based ranking with a diversity-preserving selection.
Its environmental selection is driven by two key ideas: fast non-dominated
sorting and crowding distance~\cite{deb2002fast}.

\paragraph{Fast Non-dominated Sorting.}
The combined population of parent and offspring is partitioned into a sequence of Pareto fronts based on dominance. The first front contains all
solutions that are not dominated by any other solution in the
population (the current Pareto front). The second front contains all
solutions that are only dominated by members of the first front, the
third front contains solutions dominated only by members of the first
two fronts, and so on. This yields an ordered hierarchy of fronts with
increasing dominance level. Figure~\ref{fig:fast} illustrates this idea.

\begin{figure}[h]
    \centering
    \includegraphics[width=0.5\linewidth]{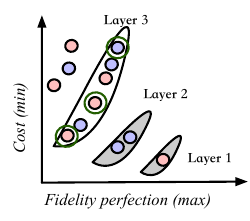}
    \caption{Illustration of fast non-dominated sorting in the objective space.}
    \label{fig:fast}
\end{figure}

\paragraph{Crowding distance.}
To maintain diversity within each Pareto front, NSGA-II assigns every
solution a crowding distance that estimates how isolated it is from its
neighbors in objective space. For each front, solutions are sorted
along each objective, boundary points are given an infinite distance,
and interior points receive the (normalized) distance to their nearest
neighbors. 

% \textbf{Illustration in this work.}
In this study, we formulate imperfect-fidelity discovering as a bi-objective problem (maximizing fidelity perfection and minimizing cost), which is optimized using NSGA-II. As illustrated in Figure~\ref{fig:fast}, parent (blue) and offspring (red) solutions (i.e., fidelity settings) are first merged and sorted into Pareto fronts. Then, the next generation is filled by taking whole fronts in order of rank until adding the next front would exceed the population size. If the last admissible front does not fit entirely, solutions in that front are sorted by crowding distance and the most isolated ones are selected (e.g., the green-circled points in Figure~\ref{fig:fast}).
