# Supplementary material for: Less Is More: Tuning Configurable Systems with Imperfect Fidelity
Source: arXiv:2608.00759 source file (2026-08-01)
Supplement: Supplementary file 7 [file section_results.tex]

\section{Results}

\begin{figure*}

    \subfloat[\textsc{MySQL}\label{fig:rq1_mysql}]{\includestandalone[width=0.64\columnwidth]{supplementary/sup_figures/mysql_single}}
    \hfill  
    \subfloat[\textsc{PostgreSQL}\label{fig:rq1_mysql}]{\includestandalone[width=0.64\columnwidth]{supplementary/sup_figures/postgresql_single}}
    \hfill  
    \subfloat[\textsc{Tomcat}\label{fig:rq1_tomcat}]{\includestandalone[width=0.64\columnwidth]{supplementary/sup_figures/tomcat_single}}
    

    \vspace{0.05cm}

    \subfloat[\textsc{Httpd}\label{fig:rq1_httpd}]{\includestandalone[width=0.64\columnwidth]{supplementary/sup_figures/httpd_single}}
    \hfill  
        \subfloat[\textsc{Gcc}\label{fig:rq1_gcc}]{\includestandalone[width=0.64\columnwidth]{supplementary/sup_figures/gcc_single}}
    \hfill  
        \subfloat[\textsc{Clang}\label{fig:rq1_clang}]{\includestandalone[width=0.64\columnwidth]{supplementary/sup_figures/clang_single}}
        
    \caption{Mean and standard deviation of performance for tuning trajectories over 10 runs.}
    \label{fig:RQ2_single}
    \vspace{-5pt}
\end{figure*}


\begin{figure*}
    \subfloat[\textsc{MySQL}\label{fig:rq1_mysql}]{\includestandalone[width=0.64\columnwidth]{supplementary/sup_figures/mysql_multi}}
    \hfill  
    \subfloat[\textsc{PostgreSQL}\label{fig:rq1_mysql}]{\includestandalone[width=0.64\columnwidth]{supplementary/sup_figures/postgresql_multi}}
    \hfill  
    \subfloat[\textsc{Tomcat}\label{fig:rq1_tomcat}]{\includestandalone[width=0.64\columnwidth]{supplementary/sup_figures/tomcat_multi}}
    

    \vspace{0.05cm}

    \subfloat[\textsc{Httpd}\label{fig:rq1_httpd}]{\includestandalone[width=0.64\columnwidth]{supplementary/sup_figures/httpd_multi}}
    \hfill  
        \subfloat[\textsc{Gcc}\label{fig:rq1_gcc}]{\includestandalone[width=0.64\columnwidth]{supplementary/sup_figures/gcc_multi}}
    \hfill  
        \subfloat[\textsc{Clang}\label{fig:rq1_clang}]{\includestandalone[width=0.64\columnwidth]{supplementary/sup_figures/clang_multi}}
        
    \caption{Mean and standard deviation of performance for tuning trajectories over 10 runs.}
    \label{fig:RQ2_multi}
    \vspace{-5pt}
\end{figure*}

\begin{figure*}
    \subfloat[\textsc{MySQL}\label{fig:rq4_mysql}]{\includestandalone[width=0.64\columnwidth]{supplementary/sup_figures/mysql_ablation}}
    \hfill  
    \subfloat[\textsc{PostgreSQL}\label{fig:rq4_mysql}]{\includestandalone[width=0.64\columnwidth]{supplementary/sup_figures/postgresql_ablation}}
    \hfill  
    \subfloat[\textsc{Tomcat}\label{fig:rq1_tomcat}]{\includestandalone[width=0.64\columnwidth]{supplementary/sup_figures/tomcat_ablation}}
    

    \vspace{0.05cm}

    \subfloat[\textsc{Httpd}\label{fig:rq4_httpd}]{\includestandalone[width=0.64\columnwidth]{supplementary/sup_figures/httpd_ablation}}
    \hfill  
        \subfloat[\textsc{Gcc}\label{fig:rq4_gcc}]{\includestandalone[width=0.64\columnwidth]{supplementary/sup_figures/gcc_ablation}}
    \hfill  
        \subfloat[\textsc{Clang}\label{fig:rq4_clang}]{\includestandalone[width=0.64\columnwidth]{supplementary/sup_figures/clang_ablation}}
        
    \caption{Mean and standard deviation of performance for tuning trajectories over 10 runs.}
    \label{fig:RQ4_ablation}
    \vspace{-5pt}
\end{figure*}
