# Supplementary material for: Less Is More: Tuning Configurable Systems with Imperfect Fidelity
Source: arXiv:2608.00759 source file (2026-08-01)
Supplement: Supplementary file 8 [file section_system_deployment.tex]

\section{Experimental Details in \approach}

% \tao{other details you can put include: options, details of how to run each of the fidelity generator, how the performance metrics are measured (note you can mention whatever library/tool you used therein.)}

% \tao{If time permitted, you might include the third part to describe step by step how to use MFtune in practice.}





\subsection{Hardware and Software Environment}
All experiments were executed on dedicated servers to avoid interference from unrelated processes. During the experiment evaluation period, no competing jobs were scheduled on the machines, and nonessential background services were disabled to eliminate performance noise.

The software environment consisted of \texttt{Python (v3.9+)} for implementing all tuners, \texttt{Docker (v24+)} for isolating target systems and ensuring reproducible execution, and \texttt{tmux} to maintain long-running sessions even under unstable SSH connections. This setup ensured consistent, uninterrupted execution during the experiment evaluation.


\subsection{System Deployment Architecture}

To guarantee clean isolation and reliable evaluation, each experiment adopts a dual-container deployment:
\begin{itemize}
    \item \textbf{System Container:} hosts the target software configurable system (e.g., \textsc{MySQL}, \textsc{PostgreSQL}, \textsc{Tomcat}, \textsc{Httpd}, \textsc{Gcc}, and \textsc{Clang}).
    \item \textbf{Tuner Container:} runs \approach~or compared tuners.
\end{itemize}

Separating the system under test from the tuner brings two benefits. First, it ensures that CPU and memory pressure caused by the tuner would not interfere with the system’s internal behavior. Second, it enables fast re-initialization: e.g., each evaluation can be conducted on a clean instance by restarting the system container, which guarantees consistency across runs and eliminates contamination from previous configurations.

\subsection{Ensuring Clean and Reproducible Evaluations}

To ensure reliable measurement, we enforce system-specific cleaning and re-initialization policies:

\begin{itemize}
    \item \textbf{Databases:} for every configuration, we instantiate a fresh database instance with a newly loaded dataset. After each evaluation, the instance is removed to avoid caching or residual state.
    \item \textbf{Web servers:} configuration changes take effect via a full restart of the system container before each evaluation.
    \item \textbf{Compilers:} configuration evaluation uses a clean container state to avoid stale build artifacts or file-system caching.
\end{itemize}

To further ensure measurement reliability, we conduct post-evaluation analysis on the collected performance data. If the measured performance (i.e., throughput and runtime) shows an abnormal scale shift---far beyond the typical range observed for the system---this often indicates interference from physical conditions such as CPU temperature variations or hardware noise. When such anomalies are detected, the entire tuning run is safely restarted to avoid contaminating the optimization process. This procedure ensures that the reported results reflect stable and reliable execution conditions. More implementation details can be found in our repository: \textcolor{blue}{\texttt{\url{https://github.com/ideas-labo/mftune}}}. 


\subsection{Fidelity Generators and Performance Measurement}
In \approach, a fidelity generator is a tool whose parameters (i.e., fidelity factors in our context) are used to shape the evaluation environment for a given configuration. By adjusting fidelity factor(s) (e.g., workload duration, request concurrency, or program complexity),  we can construct different evaluation environments (fidelity settings). For each type of target system, we adopt a standard benchmark tool and expose its most relevant parameters as fidelity factors, as detailed below. All fidelity generators are invoked via Python command-line calls (using the \texttt{subprocess} module), which also parse their standard output to extract the corresponding performance metrics.


\subsubsection{Sysbench for Database}

For \textsc{MySQL} and \textsc{PostgreSQL}, we use \textsc{Sysbench}'s OLTP benchmark as the fidelity generator. We treat \textsc{Sysbench} parameters (\texttt{tables}, \texttt{table-size}, \texttt{time}, \texttt{threads}, and \texttt{r/w ratio}) as fidelity factors. By varying these parameters, we control the data volume, transactional load, concurrency level, and read/write mix, thereby defining the fidelity setting of the database evaluation environment.

Each evaluation is executed on a freshly initialized database instance to avoid residual state. \textsc{Sysbench} is then invoked to load data and run the benchmark under the specified fidelity setting. We extract the throughput (transactions per second) from \textsc{Sysbench}’s standard output, which serves as the optimization objective for database systems.




\subsubsection{Wrk for Web Servers}
For \textsc{Tomcat} and \textsc{HTTPD}, we use \textsc{Wrk} as the fidelity generator.
The parameters (i.e., \texttt{duration}, \texttt{threads},  \texttt{connections}, \texttt{post}) act as fidelity factors. Tuning these parameters controls the length and intensity of the HTTP load as well as the request characteristics, thereby determining the fidelity setting of the web-server evaluation environment.

For each evaluation, the target web server is restarted to ensure a clean state. \textsc{Wrk} is then invoked once under the specified fidelity setting to issue HTTP requests to a fixed test endpoint. From \textsc{Wrk}’s standard output, we extract the achieved throughput (requests per second), which is used as the optimization objective for web-server systems.


\subsubsection{Csmith for Compilers}

For \textsc{GCC} and \textsc{Clang}, we use \textsc{Csmith} as the fidelity generator. 
We expose several \textsc{Csmith} parameters (e.g., \texttt{max-block-size}, \texttt{max-funcs}, \texttt{inline-function-prob}, and \texttt{max-array-len-per-dim}, and \texttt{max-block-depth}) as fidelity factors. Adjusting these parameters controls the size, structural complexity, and control-flow richness of the generated $C$ programs, and thus the fidelity setting of the compiler evaluation environment.

For each evaluation, \textsc{Csmith} generates a new $C$ program under the specified fidelity setting, and the target compiler is invoked to compile it with the candidate configuration. We then execute the compiled program and measure its runtime over the full execution process. The observed wall-clock time (runtime) is used as the optimization objective for compiler systems.


\subsection{Configuration Options}
In this study, we evaluate \approach~on six configurable systems, each of which features a distinct configuration space that can influence its performance. These spaces include both categorical options (e.g., enumerated and binary choices) and numerical options (e.g., integers and floating-point values), as commonly considered in prior work~\cite{DBLP:journals/pvldb/ZhangCLWTLC22,zhang2021restune,DBLP:journals/pvldb/KanellisDKMCV22,he2022multi,chen2021efficient}.

For each system, we select 20 representative performance-related options to form the tuning space explored in our experiments. These options cover a broad range of behaviors while keeping the search space tractable for systematic comparison. The detailed option sets for all six systems are provided in Tables~\ref{tab:mysql}-\ref{tab:clang}.
