# Supplementary material for: Less Is More: Tuning Configurable Systems with Imperfect Fidelity
Source: arXiv:2608.00759 source file (2026-08-01)
Supplement: Supplementary file 9 [file clang_knobs_table.tex]

\begin{tabular}{llll}
\toprule
\textbf{Configuration Option} & \textbf{Type} & \textbf{Default} & \textbf{Range} \\ \midrule
\texttt{fstrict-aliasing} & Categorical & Off & \{On, Off\} \\
\texttt{funroll-loops} & Categorical & Off & \{On, Off\} \\
\texttt{fno-exceptions} & Categorical & On & \{On, Off\} \\
\texttt{fomit-frame-pointer} & Categorical & Off & \{On, Off\} \\
\texttt{fno-rtti} & Categorical & On & \{On, Off\} \\
\texttt{fdata-sections} & Categorical & Off & \{On, Off\} \\
\texttt{ffunction-sections} & Categorical & Off & \{On, Off\} \\
\texttt{fmerge-all-constants} & Categorical & Off & \{On, Off\} \\
\texttt{finline-functions} & Categorical & Off & \{On, Off\} \\
\texttt{finline-small-functions} & Categorical & Off & \{On, Off\} \\
\texttt{fno-math-errno} & Categorical & On & \{On, Off\} \\
\texttt{fno-rounding-math} & Categorical & On & \{On, Off\} \\
\texttt{fno-trapping-math} & Categorical & On & \{On, Off\} \\
\texttt{fassociative-math} & Categorical & Off & \{On, Off\} \\
\texttt{freciprocal-math} & Categorical & Off & \{On, Off\} \\
\texttt{fno-signed-zeros} & Categorical & On & \{On, Off\} \\
\texttt{fno-zero-initialized-in-bss} & Categorical & On & \{On, Off\} \\
\texttt{fvectorize} & Categorical & Off & \{On, Off\} \\
\texttt{fslp-vectorize} & Categorical & Off & \{On, Off\} \\
\texttt{ftree-vectorize} & Categorical & Off & \{On, Off\} \\
\bottomrule
\end{tabular}
