# Supplementary material for: Less Is More: Tuning Configurable Systems with Imperfect Fidelity
Source: arXiv:2608.00759 source file (2026-08-01)
Supplement: Supplementary file 10 [file gcc_knobs_table.tex]

\begin{tabular}{llll}
\toprule
\textbf{Configuration Option} & \textbf{Type} & \textbf{Default} & \textbf{Range} \\ \midrule
\texttt{ffast-math} & Categorical & Off & \{On, Off\} \\
\texttt{funroll-all-loops} & Categorical & Off & \{On, Off\} \\
\texttt{fno-inline-small-functions} & Categorical & Off & \{On, Off\} \\
\texttt{finline-functions} & Categorical & Off & \{On, Off\} \\
\texttt{fno-math-errno} & Categorical & Off & \{On, Off\} \\
\texttt{fipa-cp-clone} & Categorical & Off & \{On, Off\} \\
\texttt{funsafe-math-optimizations} & Categorical & Off & \{On, Off\} \\
\texttt{fno-tree-loop-optimize} & Categorical & Off & \{On, Off\} \\
\texttt{fno-merge-constants} & Categorical & Off & \{On, Off\} \\
\texttt{fno-omit-frame-pointer} & Categorical & Off & \{On, Off\} \\
\texttt{fno-align-labels} & Categorical & Off & \{On, Off\} \\
\texttt{fno-tree-dse} & Categorical & Off & \{On, Off\} \\
\texttt{fwrapv} & Categorical & Off & \{On, Off\} \\
\texttt{fgcse-after-reload} & Categorical & Off & \{On, Off\} \\
\texttt{fno-align-jumps} & Categorical & Off & \{On, Off\} \\
\texttt{fno-asynchronous-unwind-tables} & Categorical & Off & \{On, Off\} \\
\texttt{fno-cse-follow-jumps} & Categorical & Off & \{On, Off\} \\
\texttt{fno-ivopts} & Categorical & Off & \{On, Off\} \\
\texttt{fno-guess-branch-probability} & Categorical & Off & \{On, Off\} \\
\texttt{fprefetch-loop-arrays} & Categorical & Off & \{On, Off\} \\
\bottomrule
\end{tabular}
