# Supplementary material for: Less Is More: Tuning Configurable Systems with Imperfect Fidelity
Source: arXiv:2608.00759 source file (2026-08-01)
Supplement: Supplementary file 11 [file httpd_knobs_table.tex]

\begin{tabular}{llll}
\toprule
\textbf{Configuration Option} & \textbf{Type} & \textbf{Default} & \textbf{Range} \\ \midrule
\texttt{TimeOut} & Integer & 60 & [1, 600] \\
\texttt{KeepAlive} & Categorical & On & \{Off, On\} \\
\texttt{KeepAliveTimeout} & Integer & 5 & [1, 60] \\
\texttt{MaxKeepAliveRequests} & Integer & 100 & [1, 10000] \\
\texttt{EnableSendfile} & Categorical & Off & \{On, Off\} \\
\texttt{EnableMMAP} & Categorical & On & \{On, Off\} \\
\texttt{HostnameLookups} & Categorical & Off & \{Off, On, Double\} \\
\texttt{LimitRequestBody} & Integer & 1073741824 & [0, 2147483647] \\
\texttt{LimitRequestFields} & Integer & 100 & [1, 10000] \\
\texttt{LimitRequestFieldSize} & Integer & 8190 & [0, 8190] \\
\texttt{LimitRequestLine} & Integer & 8190 & [1, 8190] \\
\texttt{ReadBufferSize} & Integer & 8192 & [1024, 65536] \\
\texttt{FlushMaxPipelined} & Integer & 5 & [-1, 1000] \\
\texttt{FlushMaxThreshold} & Integer & 65535 & [0, 1048576] \\
\texttt{RLimitCPU} & Integer & 50000 & [0, 100000] \\
\texttt{RLimitMEM} & Integer & 536870912 & [0, 1073741824] \\
\texttt{RLimitNPROC} & Integer & 512 & [0, 1024] \\
\texttt{MaxRanges} & Categorical & 200 & \{default, unlimited, none, 100, 200, 300, 500, 1000\} \\
\texttt{MaxRangeOverlaps} & Categorical & 20 & \{default, unlimited, none, 100, 200, 300, 500, 1000\} \\
\texttt{MaxRangeReversals} & Categorical & 20 & \{default, unlimited, none, 100, 200, 300, 500, 1000\} \\
\bottomrule
\end{tabular}
