# Supplementary material for: Less Is More: Tuning Configurable Systems with Imperfect Fidelity
Source: arXiv:2608.00759 source file (2026-08-01)
Supplement: Supplementary file 12 [file mysql_knobs_table.tex]

\begin{tabular}{llll}
\toprule
\textbf{Configuration Option} & \textbf{Type} & \textbf{Default} & \textbf{Range} \\ \midrule
\texttt{innodb\_thread\_concurrency} & Integer & 0 & [0, 1000] \\
\texttt{max\_allowed\_packet} & Integer & 4194304 & [1024, 1073741824] \\
\texttt{innodb\_io\_capacity\_max} & Integer & 400 & [100, 40000] \\
\texttt{tmp\_table\_size} & Integer & 16777216 & [1024, 1073741824] \\
\texttt{query\_prealloc\_size} & Integer & 8192 & [8192, 134217728] \\
\texttt{max\_heap\_table\_size} & Integer & 16777216 & [16384, 1073741824] \\
\texttt{transaction\_alloc\_block\_size} & Integer & 8192 & [1024, 131072] \\
\texttt{join\_buffer\_size} & Integer & 262144 & [128, 1073741824] \\
\texttt{innodb\_flush\_log\_at\_trx\_commit} & Categorical & 1 & \{0, 1, 2\} \\
\texttt{innodb\_max\_dirty\_pages\_pct\_lwm} & Integer & 0 & [0, 99] \\
\texttt{innodb\_buffer\_pool\_size} & Integer & 13958643712 & [10307921510, 15618062894] \\
\texttt{key\_cache\_age\_threshold} & Integer & 300 & [100, 30000] \\
\texttt{binlog\_cache\_size} & Integer & 32768 & [4096, 4294967296] \\
\texttt{innodb\_purge\_rseg\_truncate\_frequency} & Integer & 128 & [1, 128] \\
\texttt{query\_cache\_limit} & Integer & 1048576 & [0, 134217728] \\
\texttt{binlog\_row\_image} & Categorical & full & \{full, minimal, noblob\} \\
\texttt{innodb\_lru\_scan\_depth} & Integer & 1024 & [100, 10240] \\
\texttt{sort\_buffer\_size} & Integer & 262144 & [32768, 134217728] \\
\texttt{innodb\_stats\_transient\_sample\_pages} & Integer & 8 & [1, 100] \\
\texttt{innodb\_adaptive\_max\_sleep\_delay} & Integer & 150000 & [0, 1000000] \\
\bottomrule
\end{tabular}
