# Supplementary material for: Less Is More: Tuning Configurable Systems with Imperfect Fidelity
Source: arXiv:2608.00759 source file (2026-08-01)
Supplement: Supplementary file 14 [file postgresql_knobs_table.tex]

\begin{tabular}{llll}
\toprule
\textbf{Configuration Option} & \textbf{Type} & \textbf{Default} & \textbf{Range} \\ \midrule
\texttt{checkpoint\_completion\_target} & Float & 0.5 & [0.0, 1.0] \\
\texttt{backend\_flush\_after} & Integer & 0 & [0, 256] \\
\texttt{maintenance\_work\_mem} & Integer & 65536 & [1024, 1000000] \\
\texttt{max\_parallel\_workers\_per\_gather} & Integer & 0 & [0, 1024] \\
\texttt{min\_wal\_size} & Integer & 80 & [2, 8000] \\
\texttt{wal\_writer\_flush\_after} & Integer & 128 & [0, 2147483647] \\
\texttt{wal\_writer\_delay} & Integer & 200 & [1, 10000] \\
\texttt{work\_mem} & Integer & 4096 & [64, 1000000] \\
\texttt{random\_page\_cost} & Float & 4.0 & [0.0, 100] \\
\texttt{commit\_siblings} & Integer & 5 & [0, 1000] \\
\texttt{checkpoint\_flush\_after} & Integer & 32 & [0, 256] \\
\texttt{seq\_page\_cost} & Float & 1.0 & [0.0, 100] \\
\texttt{commit\_delay} & Integer & 0 & [0, 100000] \\
\texttt{join\_collapse\_limit} & Integer & 8 & [1, 2147483647] \\
\texttt{bgwriter\_delay} & Integer & 200 & [10, 10000] \\
\texttt{from\_collapse\_limit} & Integer & 8 & [1, 2147483647] \\
\texttt{default\_statistics\_target} & Integer & 100 & [1, 10000] \\
\texttt{bgwriter\_flush\_after} & Integer & 64 & [0, 256] \\
\texttt{checkpoint\_timeout} & Integer & 300 & [30, 86400] \\
\texttt{deadlock\_timeout} & Integer & 1000 & [1, 2147483647] \\
\bottomrule
\end{tabular}
