# Supplementary material for: Less Is More: Tuning Configurable Systems with Imperfect Fidelity
Source: arXiv:2608.00759 source file (2026-08-01)
Supplement: Supplementary file 15 [file tomcat_knobs_table.tex]

\begin{tabular}{llll}
\toprule
\textbf{Name} & \textbf{Type} & \textbf{Default} & \textbf{Range} \\ \midrule
\texttt{maxThreads} & Integer & 200 & [1, 20000] \\
\texttt{acceptCount} & Integer & 100 & [0, 1000] \\
\texttt{connectionTimeout} & Integer & 20000 & [1, 60000] \\
\texttt{keepAliveTimeout} & Integer & 20000 & [1, 60000] \\
\texttt{maxConnections} & Integer & 8192 & [1, 100000] \\
\texttt{minSpareThreads} & Integer & 10 & [1, 500] \\
\texttt{processorCache} & Integer & 200 & [0, 500] \\
\texttt{enableLookups} & Categorical & false & \{true, false\} \\
\texttt{asyncTimeout} & Integer & 30000 & [0, 60000] \\
\texttt{disableUploadTimeout} & Categorical & true & \{true, false\} \\
\texttt{connectionUploadTimeout} & Integer & 300000 & [0, 600000] \\
\texttt{executorTerminationTimeoutMillis} & Integer & 5000 & [0, 60000] \\
\texttt{compressionMinSize} & Integer & 2048 & [0, 100000] \\
\texttt{tcpNoDelay} & Categorical & true & \{true, false\} \\
\texttt{maxHttpHeaderSize} & Integer & 8192 & [0, 65536] \\
\texttt{maxHttpRequestHeaderSize} & Integer & 8192 & [0, 65536] \\
\texttt{maxHttpResponseHeaderSize} & Integer & 8192 & [0, 65536] \\
\texttt{maxKeepAliveRequests} & Integer & 100 & [1, 1000] \\
\texttt{threadsMaxIdleTime} & Integer & 60000 & [0, 600000] \\
\texttt{threadPriority} & Integer & 5 & [1, 10] \\
\bottomrule
\end{tabular}
